# Supplementary material for: FreeLong: Training-Free Long Video Generation with SpectralBlend Temporal Attention
Source: arXiv:2407.19918 source file (2024-07-29)
Supplement: Supplementary file 1 [file supp.tex]

\section{Appendix}

\section{Social Impacts}
It is important to consider the potential ethical implications of our approach, which is typical in generative models. By incorporating Video Diffusion Model~\cite{lavie,videocrafter} into our methodology, there is a chance that our system may also inherit the biases present in these models. Additionally, we need to be aware of the potential risks, including the generation of deceptive, harmful, or discriminatory content.

\section{Limitation}
Despite its significant advancements, FreeLong has several limitations. Temporal flickering can still occur in extended sequences, affecting the visual consistency over prolonged videos. Additionally, handling dynamic scene changes where context and content vary significantly remains challenging, as the current model may struggle to adapt to rapidly changing scenarios. Nonetheless, FreeLong represents a promising approach to training-free long-form text-to-video generation, offering significant improvements in consistency and fidelity despite these challenges.

\section{Code used and License}
\label{subsec:code}

All used codes and their licenses are listed in Table~\ref{tab:code}.

\begin{table*}[ht]
\scriptsize
\centering
\caption{The used codes and license.}

\begin{tabular}{lll}
\hline
URL & Citation & License \\ 
\hline
\url{https://github.com/Vchitect/LaVie} & \cite{lavie} & Apache License 2.0\\
\url{https://github.com/huggingface/diffusers} & \cite{diffusers} & Apache License 2.0 \\
\url{https://github.com/AILab-CVC/VideoCrafter} & \cite{videocrafter} & Apache License 2.0 \\
\url{https://github.com/modelscope/modelscope} & \cite{modelscope} & Apache License 2.0 \\
\hline
\end{tabular}
\label{tab:code}
\end{table*}

\section{More Qualitative Results}
\begin{figure*}
\centering
   \setlength{\abovecaptionskip}{0.5cm}
   \includegraphics[scale = 0.40]{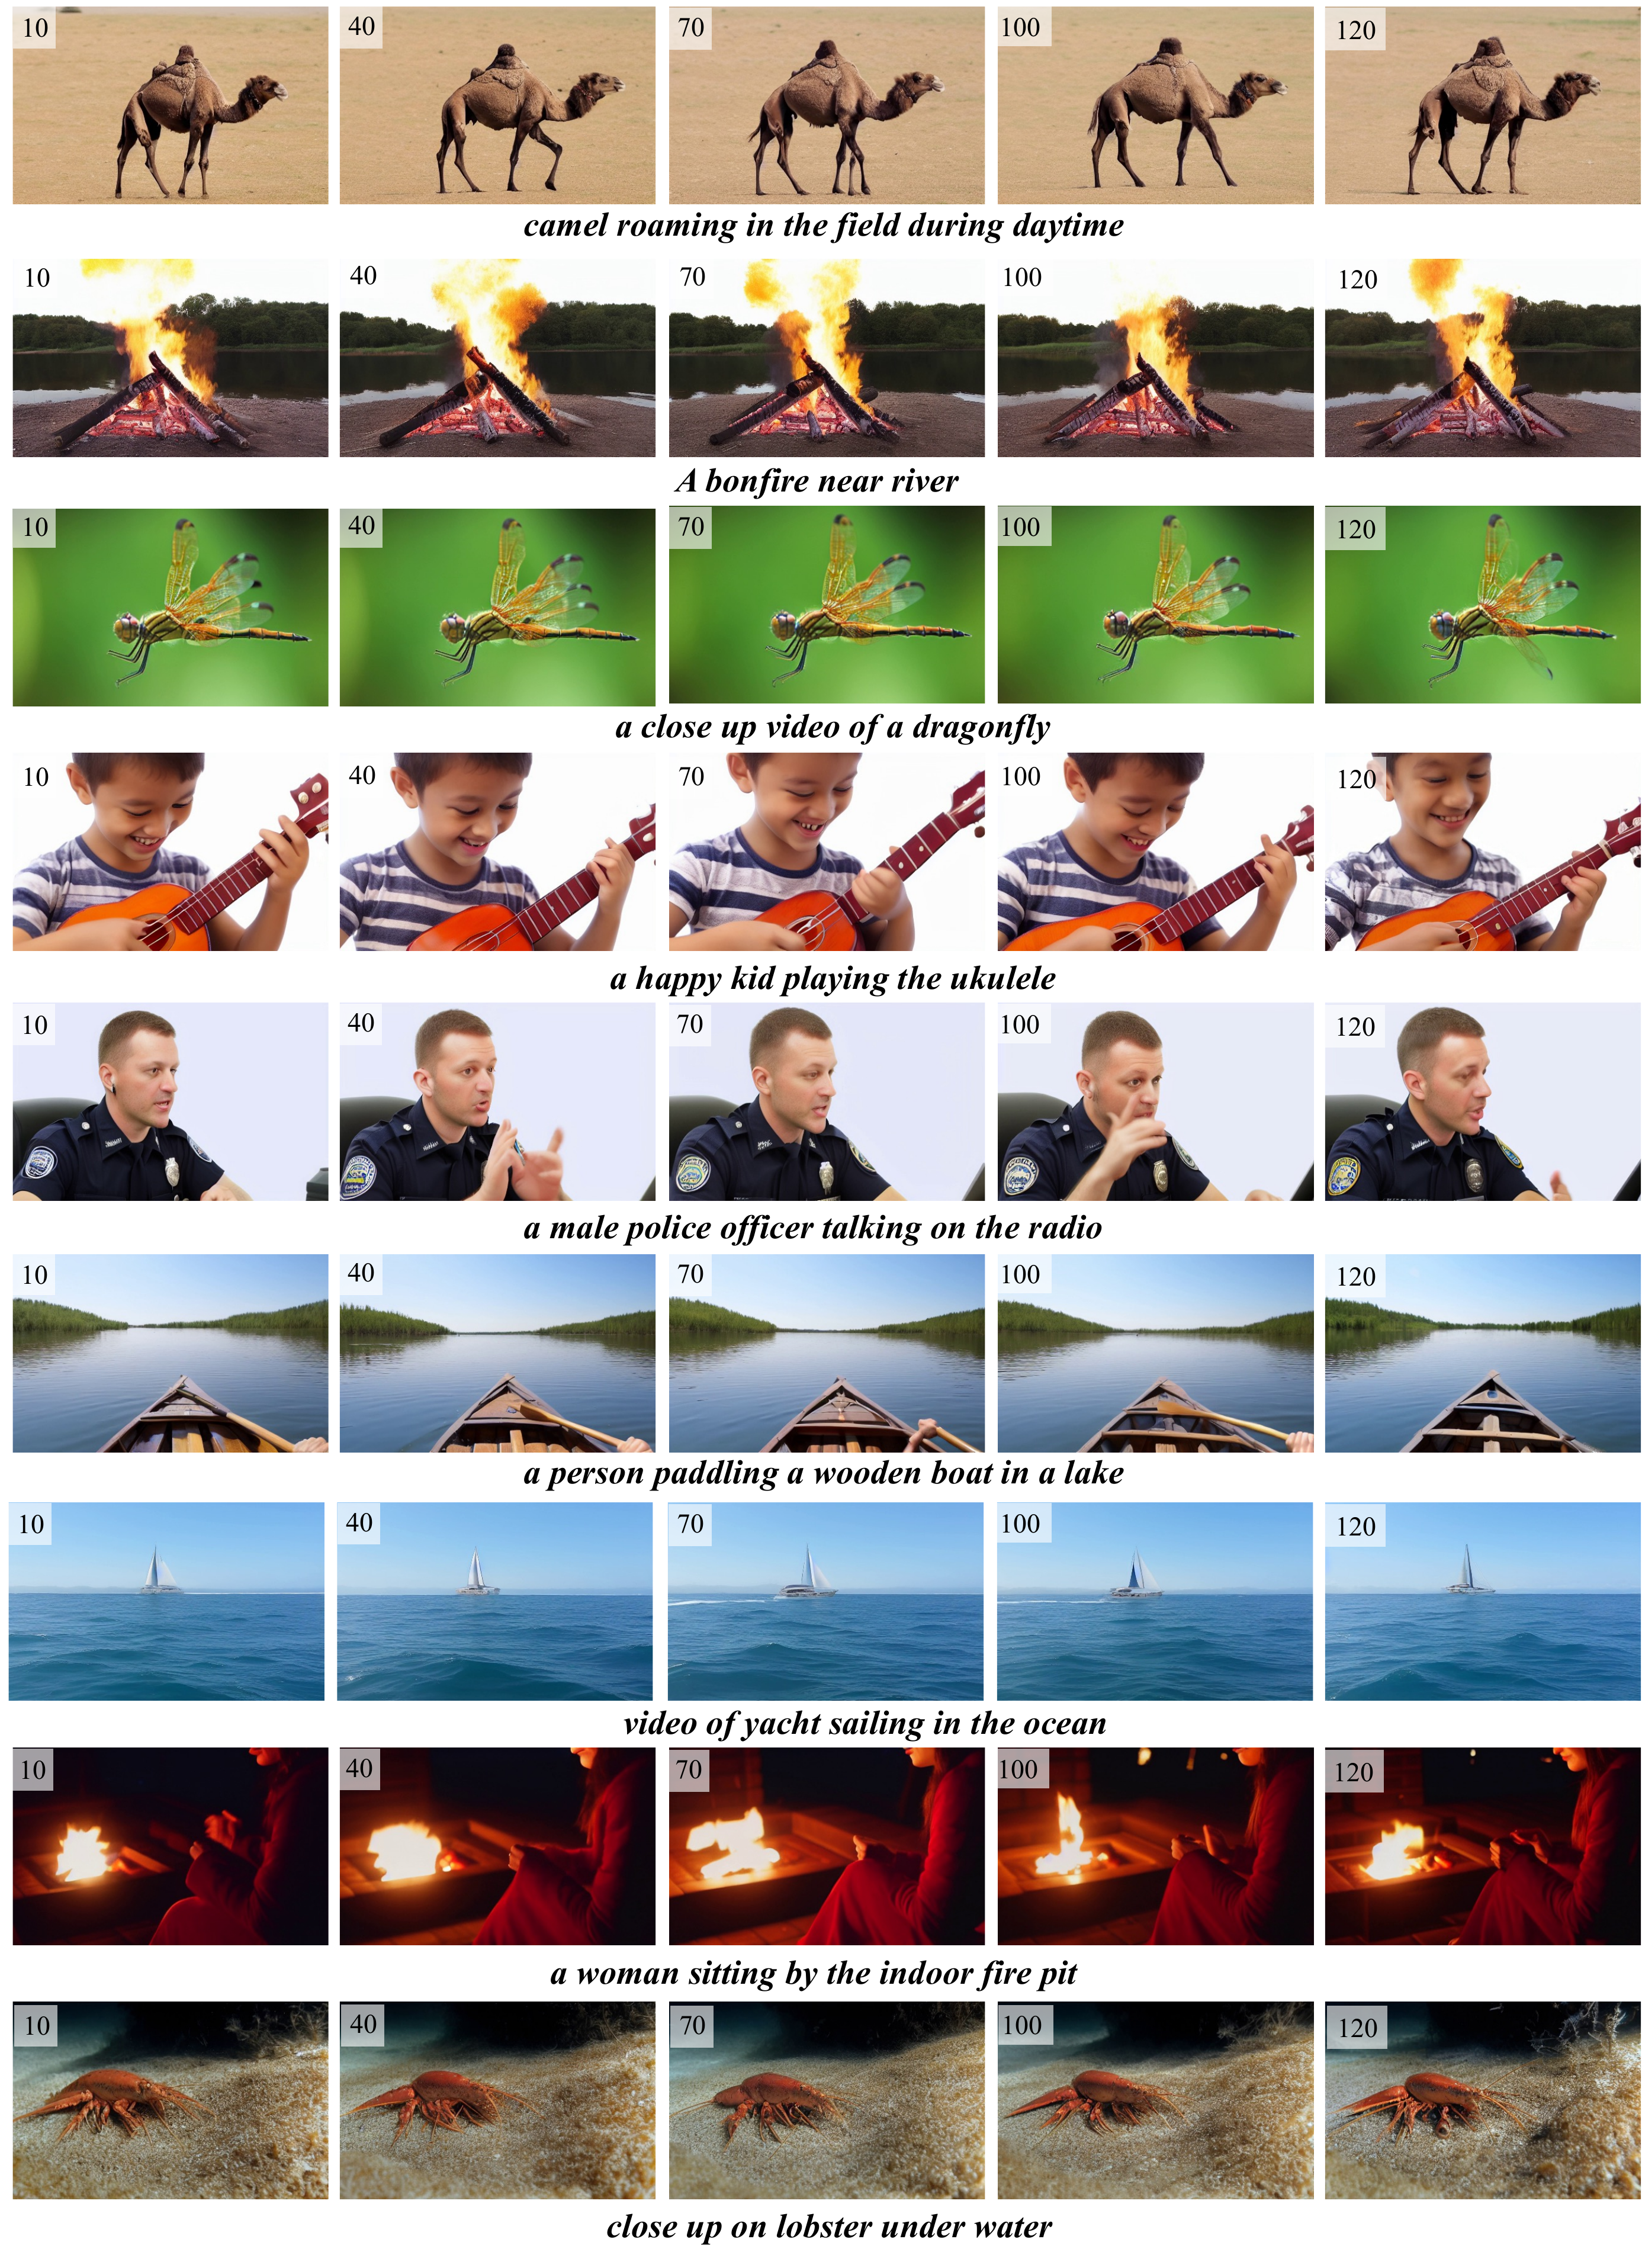}
   \vspace{-.2in}
     \caption{
\textbf{Results of Multi-Prompt Video Generation.} Our method ensures coherent visual continuity and motion consistency across different video segments.
         }
   \label{fig:multiprompt}
\end{figure*}

We add more video generation results in Figure~\ref{fig:supp}
